# Supplementary material for: Skyrmion size in skyrmion crystals
Source: arXiv:2103.13036 ancillary file (2021-03-24)
Supplement: Supplementary file 1 [file supplementary.pdf]

# Supplemental Materials: Skyrmion size in skyrmion crystals

H. T. Wu,[1,2] X. C. Hu,[1,2] K. Y. Jing,[1,2] and X. R. Wang[1,2,*]

[1]*Physics Department, The Hong Kong University of Science and Technology (HKUST), Clear Water Bay, Kowloon, Hong Kong*
[2]*HKUST Shenzhen Research Institute, Shenzhen 518057, China*

## 1. NUMERICAL EVIDENCES OF $R(n, A/D, \kappa)$

In this section, we show skyrmion size $R$ is a function of three variables, $n$, $A/D$, and $\kappa \equiv \pi^2 D^2/(16AK)$, instead of four variables in the model. We pick varied parameters in difference groups of materials and perform simulations. The three variables are fixed as $n = 1.85 \times 10^{-3}\,\mathrm{nm}^{-2}$, $A/D = 2\,\mathrm{nm}$, and $\kappa = 3$. All materials parameters in simulations varies more than 10 times.

TABLE S1. Skyrmion size with fixed A/D, n, and $\kappa$

| $A$ (pJ m$^{-1}$) | $K_1$ (kJ m$^{-3}$) | $D$ (mJ m$^{-2}$) | $M_s$(MA m$^{-1}$) | $n$ ($10^{-3}$nm$^{-2}$) | $R$ (nm) |
|---|---|---|---|---|---|
| 8 | 436.4 | 4 | 0.3 | 1.85 | 5.029 |
| 6 | 312.4 | 3 | 0.1 | 1.85 | 5.032 |
| 4 | 211.9 | 2 | 0.1 | 1.85 | 5.030 |
| 1 | 83.4 | 0.5 | 0.05 | 1.85 | 5.029 |
| 0.4 | 20.6 | 0.2 | 0.01 | 1.85 | 5.029 |

As mentioned in the main text, skyrmion sizes obtained from fitting trial spin profile are in good agreements with those obtained by measuring the radius of simulated $m_z = 0$ contours. Fig. S1 shows a $m_z = 0$ contour for a skyrmion in the SkX with the parameters of the second row in Tab. S1. By using this method skyrmion sizes in Fig. 2(a-c) are 7.16 nm, 6.24 nm, and 5.49 nm respective. The difference of the results from the two methods are less than 2%.

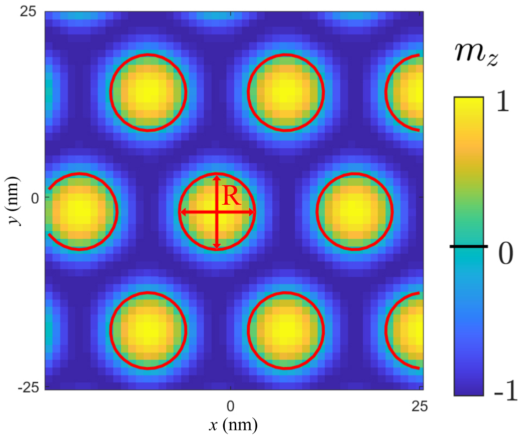


FIG. S1. Illustration of a $m_z = 0$ contour of a skyrmion and its size in the SkX with the parameters of the second row in Tab. S1. Value of size is obtained by geometric mean of R measured in two directions.

* Corresponding author: phxwan@ust.hk

## 2. DERIVATION OF SKYRMION ENERGY AND SKYRMION SIZE

We assume that an SkX is closely packed circular skyrmions in triangular lattice of lattice constant $L$. $L$ is determined by the skyrmion number density as $L = \sqrt{\frac{2}{\sqrt{3}}}\frac{1}{\sqrt{n}} \approx 1.07\frac{1}{\sqrt{n}}$. Spin profile $\Theta(r)$ of each skyrmion centred at $r = 0$ is, for $0 \le r \le L/2$,

$$\Theta(r) = 2\arctan\left\{\frac{\tan\left[\frac{\pi}{2}\cos(\frac{\pi R}{L})\right]}{\tan\left[\frac{\pi}{2}\cos(\frac{\pi r}{L})\right]}\right\}. \tag{S1}$$

Substituting $\Theta(r)$ into Eq. (1) of the main text and in the absence of the external field, energy per skyrmion $E(R)$ consists of exchange $E_{\rm ex}$, DMI $E_{\rm DM}$, and anisotropy $E_{\rm an}$ energies

$$\begin{aligned} E_{\rm ex} &= 2\pi A d\int_0^{\frac{L}{2}}\left[\left(\frac{\mathrm{d}\Theta}{\mathrm{d}r}\right)^2+\frac{\sin^2\Theta}{r^2}\right]r\mathrm{d}r \\ &= 8\pi dAf^2(\varepsilon)\int_0^1\frac{\xi^2 f'^2(\xi)+f^2(\xi)}{\xi\left[f^2(\xi)+f^2(\varepsilon)\right]^2}\mathrm{d}\xi \\ &= 2\pi dAf_1(\varepsilon), \end{aligned} \tag{S2}$$

$$\begin{aligned} E_{\rm DM} &= -2\pi Dd\int_0^{\frac{L}{2}}\left(\frac{\mathrm{d}\Theta}{\mathrm{d}r}+\frac{\sin 2\Theta}{2r}\right)r\mathrm{d}r \\ &= 2\pi dDLf(\varepsilon)\int_0^1\left\{\frac{\xi f'(\xi)}{f^2(\xi)+f^2(\varepsilon)}+\frac{f(\xi)\left[f^2(\varepsilon)-f^2(\xi)\right]}{\left[f^2(\xi)+f^2(\varepsilon)\right]^2}\right\}\mathrm{d}\xi \\ &= 2\pi dDLf_2(\varepsilon), \end{aligned} \tag{S3}$$

$$\begin{aligned} E_{\rm an} &= 2\pi Kd\int_0^{\frac{L}{2}}\sin^2\Theta r\mathrm{d}r \\ &= 2\pi dKL^2\int_0^1\left[\frac{f(\xi)f(\varepsilon)}{f^2(\xi)+f^2(\varepsilon)}\right]^2\mathrm{d}\xi \\ &= 2\pi dKL^2 f_3(\varepsilon), \end{aligned} \tag{S4}$$

where $\xi = 2r/L$, $\varepsilon = \frac{2R}{L}$, $f(\varepsilon) = \tan\left[\frac{\pi}{2}\cos(\frac{\pi}{2}\varepsilon)\right]$, and $f_i(\varepsilon)\,(i = 1, 2, 3)$ defined above are graphically plotted in Fig. S2. The

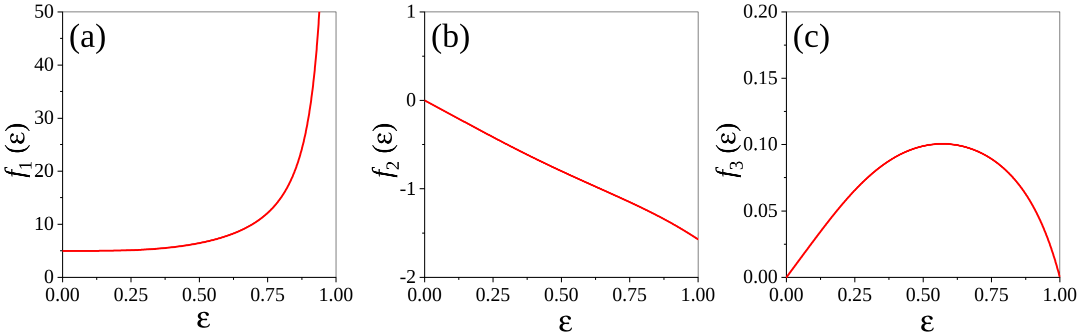


FIG. S2. Graphical plots of $f_1(\varepsilon)$ (a), $f_2(\varepsilon)$ (b), and $f_3(\varepsilon)$ (c).

energy as a function of $R$ is

$$E(R) = 2\pi d[Af_1(\varepsilon) + DLf_2(\varepsilon) + KL^2 f_3(\varepsilon)]. \tag{S5}$$

The skyrmion size $R$ is the solution of $\frac{\mathrm{d}E(R)}{\mathrm{d}R} = 0$ that is

$$2\pi d[Af_1'(\varepsilon) + DLf_2'(\varepsilon) + KL^2 f_3'(\varepsilon)] = 0, \tag{S6}$$

where $f_i'(\varepsilon)$ denotes derivatives of $f_i(\varepsilon)$ $(i = 1, 2, 3)$ with respect to $\varepsilon$. Since $f_2'(\varepsilon)$ are non-zero in $\varepsilon \in (0, 1)$, by dividing Eq. (S6) with $-Df_2'(\varepsilon)$, one has

$$\frac{A}{D}p_1(\varepsilon) + \frac{KL^2}{D}p_2(\varepsilon) - L = 0, \tag{S7}$$

where $p_1(\varepsilon) = -f_1'(\varepsilon)/f_2'(\varepsilon)$ and $p_2(\varepsilon) = -f_3'(\varepsilon)/f_2'(\varepsilon)$. Symbols in Fig. S3 are the numerical values of $p_1$ and $p_2$ that can be approximated by two analytical functions (solid curves).

$$p_1(\varepsilon) \approx -0.615 + \frac{1.883}{(1-\varepsilon)^2}, \tag{S8}$$

and

$$p_2(\varepsilon) \approx 0.611\sqrt{1-\varepsilon} - 0.404. \tag{S9}$$

Thus, equation for $R$ becomes

$$\varepsilon = 1 - \sqrt{\frac{1.883}{1 + 0.615\frac{A}{DL} - \frac{\pi^2 DL}{16A}p_2(\varepsilon)\frac{1}{\kappa}}\frac{A}{DL}}. \tag{S10}$$

$\frac{\pi^2 DL^2}{16A}p_2(\varepsilon)\frac{1}{\kappa}$ in the denominator is very small for SkXs with $\varepsilon > 0.5$. Replacing $p_2(\varepsilon)$ by $p_2(0.5)$, skyrmion size $R$, Eq. (4) in the main text, is

$$R(n, A/D, \kappa) = \frac{0.54}{\sqrt{n}} - \sqrt{\frac{0.51}{\sqrt{n}\frac{A}{D} + 0.56n\frac{A^2}{D^2} - 0.02\frac{1}{\kappa}}\frac{A}{D}}. \tag{S11}$$

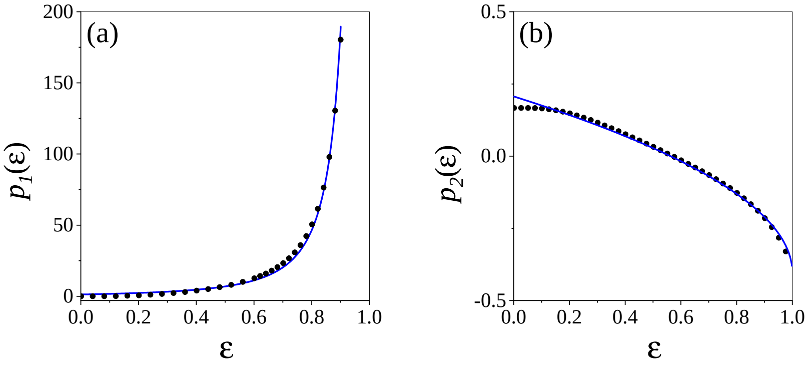


FIG. S3. Symbols are the exact values of $p_1(\varepsilon)$ (a) and $p_2(\varepsilon)$ (b) obtained numerically. Curves are the corresponding approximate functions discussed in the text.

To further demonstrate how good Eq. S11 is, we use MuMax3 to obtain skyrmion size of 180 different SkXs with model parameters in the range of $A/D = 1.25 \sim 9.16$ nm, $\kappa = 1.1 \sim 18$ and $n = 0.72 \sim 5.67\,\text{nm}^{-3}$. In Fig. S4, the x-axis is the $R$ from MuMax3, and the y-axis is computed value from Eq. S11. The fact that all points are on the red line $y = x$ proves the accuracy of size formula.

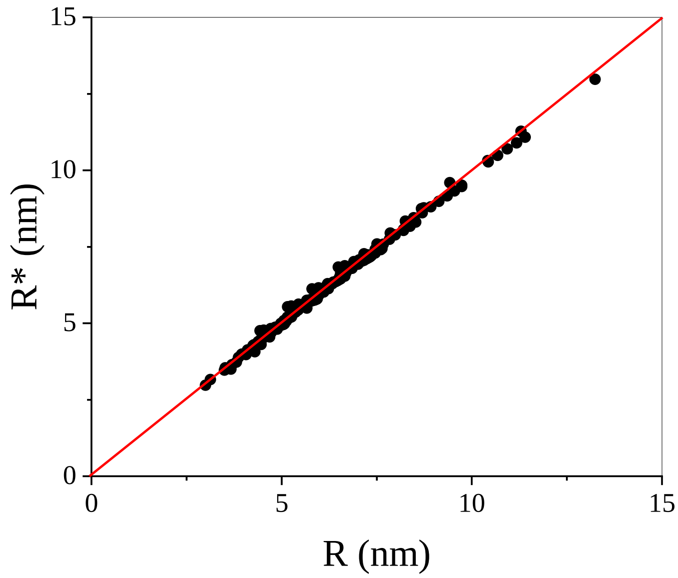


FIG. S4. The comparison of predicted sizes (y-axis) with the actual skyrmion sizes from the simulations with 180 sets of vast different model parameters.
